# Supplementary material for: Generating Diverse 3D Reconstructions from a Single Occluded Face Image
Source: arXiv:2112.00879 source file (2022-03-31)
Supplement: Supplementary file 1 [file 09-appendix_ablation.tex]

\section{Ablation Studies}\label{sec:ablation}

% \subsection{Using Mesh-VAE Decoder for Diversity Fitting}\label{subsec:ablation}
